# Supplementary material for: COSMU: Complete 3D human shape from monocular unconstrained images
Source: arXiv:2407.10586 source file (2024-07-15)
Supplement: Supplementary file 1 [file X_suppl.tex]

% \clearpage
\setcounter{page}{1}
% \title{COSMU: Complete 3D human shape from monocular unconstrained images}
% \maketitlesupplementary
\section{Overview}
In the following sections, we present additional information that supplements the main paper. Additional details on the implementation of COSMU are presented in~\cref{ssec:implementation}. A pseudocode of COSMU algorithm is outlined in~\cref{ssec:pseudo}. Examples of limitations of COSMU are shown in~\cref{ssec:limitation} while~\cref{ssec:ablation3} presents an additional study on the level of similarity between target and reference images.~\cref{ssec:ablation4} shows results obtained with six views as input to the multi-view attention-based implicit model. Examples of 3D shapes reconstructed directly from registered point clouds rather than generating and processing 2D normal maps are illustrated in~\cref{ssec:ablation5}.  2D normal maps generated by different configurations of the multi-view scenario simulation module presented in~\cref{ssec:ablation} of the main paper are illustrated in~\cref{ssec:ablation2}. A summary of the notation used in the main paper is presented in~\cref{ssec:notations}. Finally, additional results are shown in~\cref{ssec:additional}
\section{Implementation details}
\label{ssec:implementation}
\begin{figure*}[t]
\centering
\includegraphics[width=0.85\linewidth]{figures/supplementary/networks.pdf}
\caption{(a) $f_c$ implicit model to estimate coarse point clouds $\zeta$ from an input image $I$; (b) $f_{\zeta}$ implicit model to estimate the 3D body parts $\upsilon$ of a point cloud $\zeta$; (c) $f_f$ multi-view attention-based implicit model to estimate the occupancy of the complete shape.}
\label{fig:networks}
\end{figure*}
To extract segmentation masks from the input image we use the method presented by K. Lin \etal~\cite{lin2020cross} whilst 3D poses are estimated with the work by W. Li \etal~\cite{li2022mhformer}. We apply FilterReg~\cite{gao2019filterreg} to compute the rotation matrix $R$ and translation $T$.
\\ $\bullet f_{c}$: The neural implicit model $f_{c}$ (\cref{fig:networks}a) used to create the coarse point clouds $\zeta$, is trained with images of size ($N_I  \times N_I, N_I = 512$) obtained by downscaling ground truth images $I_{HR}$ by a factor of 2 with bicubic degradation. $N_T = 24000$ 3D points $X_c$ are sampled with a mixture of uniform sampling and importance sampling around the ground-truth surface following PIFu~\cite{saito2019pifu}. A subset of $X_c$ of $N = 6000$ points is selected for training. Input images are processed by a U-net (\cref{tab:unet}) that aims to increase the resolution of the feature to encode high-frequency details. High-resolution features $\phi(I)$ of size  ($1024\times1024\times64$) and low-resolution features of size ($256\times256\times256$) to enable holistic reasoning are extracted by the U-Net and processed by a stacked
hourglass architecture, which has been proven to be efficient for surface reconstruction~\cite{saito2019pifu}. We adopt 4 stacks of the stacked hourglass network~\cite{newell2016stacked} with modifications proposed by~\cite{jackson20183d}. The subset of $X_c$ points is projected on the input image and indexed to the high-resolution and low-resolution features. The concatenation of the indexing is processed by the MLP.
%The outputs of the image feature extractor of $f_{\zeta}$ are an HR feature vector of size ($2N_I \times 2N_I \times 64$) and a LR one of size ( $\frac{N_I}{1} \times \frac{N_I}{1} \times 256$). 
To model the implicit function, the MLP of $f_{c}$ has the number of neurons of (321, 1024, 512, 256, 128, 1) with skip connections at 3rd, 4th and 5th layers. 
\\ $\bullet f_{\zeta}$: The same images and 3D ground-truth of $f_c$ are used to train $f_{\zeta}$, which is showed in~\cref{fig:networks}b. Semantic masks are extracted and concatenated to the RGB image and used as input of $f_{\zeta}$. Since the objective of this neural model is to classify 3D points of a point cloud $\zeta$, instead of sampling 3D points around the ground-truth surfaces as for $f_c$, we sampled $N = 8000$ 3D points  $X_{\zeta}$ on the surface of the 3D ground-truth shapes. 4 stacks of the stacked hourglass architecture are used to extract the features from the input RGB image concatenated with the segmentation mask $I||M$.
%The output of the image feature extractor of $f_{\zeta}$ is a feature vector of size ($128 \times 128 \times 256$) and 
\begin{table}[t!]
\centering
\caption{U-Net architecture used as feature extractor of $f_c$.The output of layer 26 is the low-resolution feature while the output of layer 30 is the high-resolution one.}
\resizebox{0.95\linewidth}{!}{\input{tables/supplementary/unet}}
\label{tab:unet}
\end{table} 
The MLP has the number of neurons of (257, 1024, 512, 256, 128, 10) with skip connections at 3rd, 4th and 5th layers.
\\ $\bullet f_f$:
For the multi-view attention-based implicit model $f_f$, showed in~\cref{fig:networks}c, we apply the reference selection algorithm to select $N_r=3$ 2D normal maps of size 512x512 for each of the 360 views generated from the THuman2.0 dataset~\cite{tao2021function4d}. Having 4 views of the model ensures complete visibility of the entire surface of the model. We train the multi-view implicit model by sampling the shapes as done for training $f_{c}$. \\Firstly, the multi-view attention-based model extracts features from each input normals using 4 stacks of the stacked hourglass architecture. Then, a standard multi-head transformer-style architecture is applied~\cite{vaswani2017attention}, as shown in~\cref{fig:networks}c.  Given three vectors query
$Q = M_q\phi$, key $K = M_k\phi$, and value $V = M_v\phi$ as the embedding of the original feature $\phi$ and parameterized by matrices $M_q$, $M_k$ and $M_v$, an attention score is computed for each view $v$ based on the compatibility of a query with a corresponding key:
\begin{equation}
    Attention(Q,K,V)=softmax\left(\frac{QK^T}{\sqrt{d_k}}\right)V
\end{equation}
where $d_k$ is the common dimension of $K$, $Q$ and $V$.
Multiple heads are used to generate the $N_r+1$ features for each view as:
\begin{equation}
\begin{gathered}
    MultiHead(Q, K, V)=concat(H_1, ..., H_h)W^o
    \\
    H_i=Attention(QW^q_i, KW^k_i,V W^v_i)
\end{gathered}
\end{equation}
where $QW^q_i, KW^k_i,V W^v_i$ are the parameters of $Q$, $K$ and $V$, and $W^o$ the parameters of the final projection. The final feature is computed with the mean of the processed features. Each one of these features contains the original information from the corresponding view $v$ plus the information from all the other available views.
Refer to~\cite{vaswani2017attention} for additional details. 
The MLP that processes the final feature has the number of neurons of (257, 1024, 512, 256, 128, 1) with skip connections at 3rd, 4th and 5th layers.
\\To train all the models, Adam optimizer is adopted with a learning rate of $1e-4$ and the batch size has been set to 8. The inference time for one image of each models, without code optimization, is in the order of the second.
\\For the experiments, we set $N_r=3$, such that $v=4$ views of the subject are processed by the multi-view attention-based implicit model. Consequently, the central angles of each group $r=1, 2, 3$ are $\theta^1_c=90\degree, \theta^2_c=180\degree, \theta^3_c=270\degree$. The groups are created by adding the reference images to the group considering the orientation angle $\theta_u$:
\begin{equation}
\label{eq:grouping}
\begin{gathered}
    I^m_u \in G_r \quad\quad\quad if \quad\theta^r_{u} \in [\theta^r_c-\alpha, \theta^r_c+\alpha]\\
    \alpha=\frac{360}{2(N_r+1)}
    \end{gathered}
\end{equation}
where $G_r$ is the $r^{th}$ group of unconstrained images, $m \in [1,...,N_u]$ and $r \in [1,..., N_r]$.  $N_g$ varies for each group depending on the number of unconstrained images $I^g_u$ that are classified for the specific group.
\\It is important to notice that the unconstrained images are clustered into $N_r$ groups considering their orientation with the target body before applying the energy optimization algorithm. This is to ensure that $N_r$ references showing the entire body are selected. Without this step, for example, given a front target image, the reference selection will be biased towards unconstrained images showing the full back-view of the individual due to the visibility criterion. This criterion prioritizes unconstrained images where the body parts are more visible, counting the number of pixels of the body part in the semantic mask. In a back-view image of the subject, the torso is significantly more visible than in a side-view. If the initial clustering is not performed, that reference will always have a higher value for visibility, risking that side views will not be selected. 
\section{Algorithm for COSMU}
\label{ssec:pseudo}
To facilitate the understanding of the multi-view scenario simulation module, we include the algorithm of COSMU (Alg.~\ref{alg:pseudo}). Set notation is used in the pseudocode. 
\begin{algorithm*}

\caption{COSMU ALGORITHM}
\begin{algorithmic}[1]

\State Retrieve $\zeta_t$ from $I_t$ by estimating $\hat{s}_{c}$ with~\cref{eq:coarse_point}
\State Retrieve $\{\upsilon^p_t\}^{N_p}_{p=1}$ of $\zeta_t$ by estimating $\hat{s}_{\zeta}$ with~\cref{eq:part_class}
\State Create 2D normal map $S_0$ from $\zeta_t$
% \COMMENT $N_u$ unconstrained images $I_u$ are clustered into $N_r$ groups considering their orientation angle with the target image
\For{i = 1:$N_u$ (for all the unconstrained images)}
\State Add $I^i_u$ to a group $G^r$  with~\cref{eq:grouping} as: $G^r=\{I^g_u\}^{N_g}_{g=1},\quad g \in [1,\ldots,N_g],\quad r \in [1,\ldots,N_r]$
\EndFor

\For{$r$ = 1:$N_r$ (for all the groups)}

% \COMMENT $N_p$ references images $I_{ref}^{p,r}$ are selected for each body part for the $r^{th}$ group  via body part-based reference selection
\State $\{I^{\{p,r\}}_{ref}\}^{N_p}_{p=1}$ =\Call{ReferenceSel}{$\{I^{\{g,r\}}_{u}\}^{N_g}_{g=1}$}
% \COMMENT The selected $N_p \times N_r$ references images $\{\{I^{p,r}_{ref}\}^{N_p}_{p=1}\}^{N_r}_{r=1}$  are processed by the body part-based registration to estimate a 2D normal maps $S_v$ registered with the target input.
\State $S_r=$\Call{PartReg}{$\{I^{\{p,r\}}_{ref}\}^{N_p}_{p=1}, \{\upsilon^p_t\}^{N_p}_{p=1}$}
\EndFor
\State Estimate $\hat{s}_f$ with $f_f$ from the obtained $S_v=\left\{S_0,\{S_r\}^{N_r}_{r=1}\right\}, v \in [1, \ldots, N_r+1]$ with~\cref{eq:final_estimation}
\Statex

\Function{ReferenceSel}{$I_u$} 
\For{p = 1:$N_p$ (for all the body parts)}
\For{g = 1:$N_g$ (for all the images of a specific group)}
\State Compute $o_g$ with~\cref{eq:orientation}
\State Compute $v_g^{p}$ with~\cref{eq:visibility}
\State Compute $b_g^{p}$ with~\cref{eq:similarity}
\EndFor
\For{K in $[o, v^p, b^p]$:}
\If{$K==o$ or $K==b^p$:}
    \State Sort $\{I^g_u\}^{N_g}_{g=1} \quad \rightarrow \quad K=\{I^1_u,...,I^{N_g}_{u}\},\quad K(I^1_u) \leqslant \ldots \leqslant K(I^{N_g}_u)$.
\Else
    \State Sort $\{I^g_u\}^{N_g}_{g=1}\quad \rightarrow \quad K=\{I^1_u,...,I^{N_g}_{u}\},\quad K(I^1_u) \geqslant \ldots\geqslant K(I^{N_g}_u)$.
\EndIf
\EndFor
\State $I^{p}_{ref}=\argmin_{g}(E^{p}_{g})$ with~\cref{eq:energy} where $E^p_g=\idx_{I_u^g}(K=o)+\idx_{I_u^g}(K=v^p)+\idx_{I_u^g}(K=b^p)$
\EndFor
\State\Return $\{I^{p}_{ref}\}^{N_p}_{p=1}$
\EndFunction
\Statex
\Function{PartReg}{$I_{ref}, \upsilon_t $} 
\For{p = 1:$N_p$ (for all the body parts)}
\State Retrieve $\zeta^p_{ref}$ from $I^p_{ref}$ by estimating $\hat{s}_{c}$ with~\cref{eq:coarse_point} 
\State Retrieve $\upsilon^p_{ref}$ from $\zeta^p_{ref}$ by estimating $\hat{s}_{\zeta}$ with~\cref{eq:part_class}
\State Register $\upsilon^p_{ref}$ with $\upsilon^p_t$ as $\upsilon^p_{reg}=R(\upsilon^p_{ref})+ T $ 
\EndFor
\State Combine the $N_p$ registered body parts $\{\upsilon^p_{reg}\}^{N_p}_{p=1}$ into a point cloud $\zeta_f$
\State Create 2D normal map $S$ from the registered point cloud  $\zeta_f$
\State\Return $S$
\EndFunction

% Three sorted vectors are obtained, one for each metric.  
%     % \begin{itemize}
%     \\$\bullet$ vector $o=[r_1, r_3, r_2,..., r_4],\resizebox{0.4\hsize}{!}{$o^{r_1} \leqslant o^{r_3} \leqslant o^{r_2} \leqslant o^{r_4}$}$
%     \\$\bullet$ vector $b=[r_2, r_1, r_4,..., r_3],\resizebox{0.4\hsize}{!}{$ b^{r_2} \leqslant b^{r_1} \leqslant b^{r_4}  \leqslant b^{r_3}$}$
%     \\$\bullet$ vector $v=[r_3, r_1, r_2,..., r_4],\resizebox{0.4\hsize}{!}{$ v^{r_3} \geqslant v^{r_2} \geqslant v^{r_1} \geqslant v^{r_4}$}$
% \State Compute $r^j_k$ with~\cref{eq:energy}.
% \\$r^j_k=\argmin_{r}\left(E^{j}_{k}(r)\right)=r_1$ since $min\left(E^{j}_{r}(r)\right)=2$ \rightarrow $E^j_k(r_1)=2 \rightarrow  idx_{min}(o^{r_1})=0 + idx_{max}(v^{r_1})=1 + idx_{min}(s^{r_1})=1$; 

% \State Divide $N_M$ reference images in $N_R$ parts
% \State Extract feature vectors of reference image parts $\phi^r(I_{ref}^m)$
% \State Extract feature vectors of LR input $\phi(I_{LR})$
% \State Divide $\phi(I_{LR})$ into $N_C$ subvectors $\rightarrow \{\phi^c(I_{LR})\}^{N_C}_{c=1}$ 

% \For{m = 1:$N_M$ (for all the references)}

\end{algorithmic}

\label{alg:pseudo}
\end{algorithm*}
\section{Limitations}
\label{ssec:limitation}
\begin{figure*}[t]
\centering
\includegraphics[width=0.85\linewidth]{figures/supplementary/limitation.pdf}
\caption{Limitations of COSMU: (a) Reconstruction by leveraging a collection of images where the back is not visible. (b) Reconstruction leveraging unconstrained images with significantly different poses compared to the target one. (c) Low quality in small regions such as face and hands.}
\label{fig:limitation}
\end{figure*}
As explained in~\cref{sec:4_experiments} of the main paper, one of the limitations of COSMU is its contingency to the unconstrained images. If some body parts are not visible in the unconstrained images, then details of those regions cannot be represented by COSMU. To show this, we remove all the unconstrained images showing a back view of the subject.~\cref{fig:limitation}a illustrate the reconstructed 3D shape, which lacks of details in the back. Other parts of the body are influenced as well since the references selected for the group with $\theta_c^r=180\degree$ do not show the back view for any body part, influencing pixel-alignment.
\\Another problem related to the selection of references arises when these are significantly different from the target.~\cref{fig:limitation}b shows an example where the pose of the target and the poses of the unconstrained images are significantly different, deteriorating the performance of the body part-based registration algorithm. 
\\For some examples, COSMU cannot reproduce the same high-quality level in small regions of the human body as shown in~\cref{fig:limitation}c, where the quality of the clothing is significantly higher than the quality of the face.
\section{Similarity between references and target images}
\label{ssec:ablation3}
\begin{figure*}[t]
\centering
\includegraphics[width=0.85\linewidth]{figures/supplementary/ablation3_new.pdf}
\caption{Different results obtained by leveraging reference images of different levels of similarity with the target.}
\label{fig:similarity}
\end{figure*}
As explained in~\cref{ssec:limitation}, COSMU is influenced by the nature of the unconstrained images of the input collection. We propose an additional study to show the importance of the unconstrained images. In THuman3.0~\cite{deepcloth_su2022} there are few models captured in different clothing. Starting from these, we define 4 different collections of unconstrained images: (1) the collection is composed of unconstrained images of a different individual. This represents the set with the lowest level of similarity between the target image and the references. It is important to notice that leveraging unconstrained images of a different individual is beyond the scope of this work but we still show results for completeness. (2) Unconstrained images of the same individual with different poses and clothing are considered. (3) The collection is created with unconstrained images of the same individual in different poses but with the same clothing. (4) As in the multi-view scenario, images of the same subject in the same pose and clothing are included in the collection.~\cref{fig:similarity} shows the shapes reconstructed by COSMU with the four sets of unconstrained images. As expected, the best results, with a similar level of quality as ground-truth, are obtained when the poses and clothing are the same for the target and the unconstrained images (case 4). This is the ideal case of a multi-view scenario and these images can only be captured with inaccessible systems. The lowest quality reconstruction is obtained with case 1 when the subject of the unconstrained images differs from the subject of the target image. The different size of the human body parts of the target and reference individuals deteriorates the performance of the multi-view scenario simulation module, reducing the quality of the final reconstruction. 
\\We did not perform a quantitative study because there is not a sufficient number of 3D models of the same subject in different clothing in THuman3.0~\cite{deepcloth_su2022}.
\section{Number of selected references}
\label{ssec:ablation4}
\begin{table}[!]
\centering
\caption{Quantitative results obtained by reconstructing the 3D shapes with different numbers of views as input to the multi-view attention-based implicit model.}
\resizebox{0.95\linewidth}{!}{\input{tables/supplementary/REF5}}
\label{tab:ref5}
\end{table} 
\begin{figure}[!]
\centering
\includegraphics[width=1\linewidth]{figures/supplementary/ablation2_ref.pdf}
\caption{3D shape reconstructed by selecting different numbers of views as input to the multi-view attention-based implicit model. The same example of~\cref{fig:comparisons} of the main paper is shown to compare the reconstructions with the other approaches. Front, back, left and right side views are shown.}
\label{fig:ref5}
\end{figure}
In the main paper (\cref{ssec:comparison_cosmu}), we present results obtained by changing the number of selected references $N_r$, including results for $N_r=0$ (Baseline), $N_r=1$ (COSMU-2) and $N_r=3$ (COSMU). For completeness, we extend the analysis to $N_r=5$ where six views are used in the final reconstruction.~\cref{fig:ref5} shows the 3D shapes reconstructed from different numbers of views obtained with the multi-view scenario simulation module. The highest quality shapes are obtained when higher numbers of views are leveraged (4 and 6 views), highlighting the importance of having a complete view of the body in the reference images. This result is confirmed quantitatively in~\cref{tab:ref5}. With only one view, the regions of the body not represented in the target image appear smooth and lack fine details. When two views are used, the sides of the 3D shape are noisy and overly smoothed. A complete and high-quality representation of the entire body is achieved only when four or more images are selected as references. Notably, the 3D shape reconstructed with 6 views is slightly noisier than the one obtained using 4 views. This is due to the fact that some regions of the human body overlap across the multiple input views, introducing artifacts in the reconstruction. Since the computational resources increase with the number of views, we opt to use 4 views as the primary model.
\begin{figure*}[!]
\centering
\includegraphics[width=\textwidth,height=0.99\textheight,keepaspectratio]{figures/supplementary/directly.pdf}
\caption{3D meshes reconstructed by applying Alpha-Shape~\cite{edelsbrunner1983shape} and Ball Pivoting~\cite{bernardini1999ball} algorithms to the registered point clouds obtained with the body part-based registration step. Front, back, left and right side views are shown.}
\label{fig:directly}
\end{figure*}
\section{Reconstruction from registered point cloud}
\label{ssec:ablation5}
As explained in~\cref{sec:3_methods} of the main paper, 2D normal maps are generated from the registered point clouds $\zeta_f$ created with the body part-based registration process and processed by a multi-view implicit model that reconstructs the final 3D shape. The direct reconstruction of a 3D mesh from the multi-view point clouds $\zeta_f$ proves challenging due to the absence of known correspondences between the point clouds. Consequently, the effective application of fusion algorithms becomes impractical. The sole method for directly retrieving a 3D mesh from the registered point clouds $\zeta_f$ involves concatenating all points from these point clouds into a single point cloud. Subsequently, either the ball-pivoting~\cite{bernardini1999ball} or the alpha-shape~\cite{edelsbrunner1983shape} algorithms can be applied to create the 3D mesh. However, as illustrated in~\cref{fig:directly}, these approaches result in a loss of fine details and the quality of the 3D shapes is significantly lower when compared to the ones obtained by COSMU. This degradation in quality can be attributed to the fact that, within a single registered point cloud, only one side represents high-quality information, while the remaining sides are smooth. When merged with other views, the smooth sides influence the overall quality of the high-quality sides, leading to a final lower-quality 3D shape. 
\section{Additional results to Ablation Study}
\label{ssec:ablation2}
\begin{figure*}[!]
\centering
\includegraphics[width=0.85\linewidth]{figures/ablation2_norm.pdf}
\caption{Multi-view normal maps resulting from different configurations of the body part-based registration module. 4 views are shown (front, back, left and right side).}
\label{fig:ablation_norm}
\end{figure*}
In the second ablation study of the paper (\cref{ssec:ablation}), we show the resulting 3D shapes obtained with the multi-view attention-based implicit model from $N_r+1$ 2D normal maps generated with different configurations of the body part-based registration stage of COSMU.
\\We decided to generate normal maps instead of RGB images in order to avoid the challenging task of estimating color values for each 3D point of the point clouds. Moreover, operating in the normal space allows to choose unconstrained images of the subject in different clothing.
\cref{fig:ablation_norm} illustrates the 2D normals obtained with the different configurations. The configuration adopted by COSMU can generate noise-free normal maps compared to the ones generated by other configurations, which present severe artifacts. The second-best normal maps are obtained by the \textbf{Average} configuration, demonstrating the importance of performing a body part-based registration.
\section{Notations}
\label{ssec:notations}
To facilitate the understanding of the main paper,~\cref{tab:notation} presents a list of the notations used in the paper.
\begin{table}[!]
\centering
\caption{List of notations used in the main paper.}
\resizebox{0.85\linewidth}{!}{\input{tables/supplementary/notations}}
\label{tab:notation}
\end{table} 
\section{Additional results}
\label{ssec:additional}
\cref{fig:supp1} and~\cref{fig:supp2} present the results for the other methods that are not shown in~\cref{fig:comparisons} of the main paper. Although these methods can reproduce details in the visible parts of the input image, the quality of the non-visible regions is significantly lower than the one of the 3D shapes reconstructed with COSMU. COSMU-2 is the only other approach that can represent high-quality details in the occluded regions of the body. However, COSMU-2 exhibits artefacts and excessive smoothing on the sides of the shapes, demonstrating the benefit of leveraging references showing the entire body as in COSMU.~\cref{fig:supp3} and~\cref{fig:supp4} further demonstrate the superiority of COSMU over all the tested approaches showing new results with unconstrained images taken from the same scenarios as~\cref{fig:comparisons} of the main paper. COSMU ability to reproduce higher-quality details in non-visible regions is shown also in the examples of 3D human shapes reconstructed from images taken from the X-Human dataset~\cite{shen2023x} in~\cref{fig:supp5}. 
\\\cref{fig:reference3} and~\cref{fig:reference4} shows the $N_p \times N_r$ reference images selected by the body part-based reference selection and used in the reconstruction process for~\cref{fig:comparisons} of the main paper.~\cref{fig:reference1} shows the references selected for~\cref{fig:supp3} while~\cref{fig:reference2} for~\cref{fig:supp4}. 
\\Finally,~\cref{fig:ground-truth} illustrates the ground-truth 3D shapes for the models reconstructed with COSMU used in the main paper. Only the data from THuman3.0~\cite{deepcloth_su2022} are shown since all the other 3D shapes are reconstructed from real images and 3D ground-truth is missing.
\begin{figure*}[t]
\centering
\includegraphics[width=\textwidth,height=0.99\textheight,keepaspectratio]{figures/supplementary/supp1.pdf}
\caption{3D shapes reconstructed with related works of COSMU in several scenarios. Front, back, left and right side views are shown.}
\label{fig:supp1}
\end{figure*}
\begin{figure*}[t]
\centering
\includegraphics[width=\textwidth,height=0.99\textheight,keepaspectratio]{figures/supplementary/supp2.pdf}
\caption{3D shapes reconstructed with related works of COSMU in several scenarios. Front, back, left and right side views are shown.}
\label{fig:supp2}
\end{figure*}
\begin{figure*}[t]
\centering
\includegraphics[width=\textwidth,height=0.99\textheight,keepaspectratio]{figures/supplementary/supp4.pdf}
\caption{Additional comparisons of COSMU with related works in several scenarios. Front, back, left and right side views are shown.}
\label{fig:supp3}
\end{figure*}
\begin{figure*}[t]
\centering
\includegraphics[width=\textwidth,height=0.99\textheight,keepaspectratio]{figures/supplementary/supp3.pdf}
\caption{Additional comparisons of COSMU with related works in several scenarios. Front, back, left and right side views are shown.}
\label{fig:supp4}
\end{figure*}
\begin{figure*}[t]
\centering
\includegraphics[width=\textwidth,height=0.99\textheight,keepaspectratio]{figures/supplementary/xhuman.pdf}
\caption{Examples of 3D human shapes reconstructed from images of X-Humans dataset~\cite{shen2023x}. Front, back, left and right side views are shown.}
\label{fig:supp5}
\end{figure*}
\begin{figure*}[t]
\centering
\includegraphics[width=\textwidth,height=0.95\textheight,keepaspectratio]{figures/supplementary/references3.pdf}
\caption{$N_p \times N_r$ reference images selected by the body part-based reference selection algorithm for the examples in~\cref{fig:comparisons} of the main paper.}
\label{fig:reference3}
\end{figure*}
\begin{figure*}[t]
\centering
\includegraphics[width=\textwidth,height=0.95\textheight,keepaspectratio]{figures/supplementary/supp6.pdf}
\caption{$N_p \times N_r$ reference images selected by the body part-based reference selection algorithm for the examples in~\cref{fig:comparisons} of the main paper.}
\label{fig:reference4}
\end{figure*}
\begin{figure*}[t]
\centering
\includegraphics[width=\textwidth,height=0.95\textheight,keepaspectratio]{figures/supplementary/reference1.pdf}
\caption{$N_p \times N_r$ reference images selected by the body part-based reference selection algorithm for the examples in~\cref{fig:supp3}.}
\label{fig:reference1}
\end{figure*}
\begin{figure*}[t]
\centering
\includegraphics[width=\textwidth,height=0.95\textheight,keepaspectratio]{figures/supplementary/supp5.pdf}
\caption{$N_p \times N_r$ reference images selected by the body part-based reference selection algorithm for the examples in~\cref{fig:supp4}.}
\label{fig:reference2}
\end{figure*}
\begin{figure*}[t]
\centering
\includegraphics[width=\textwidth,height=0.99\textheight,keepaspectratio]{figures/supplementary/ground-truth.pdf}
\caption{3D shapes ground-truth of the subjects reconstructed with COSMU from THuman3.0~\cite{deepcloth_su2022}. Front, back, left and right side views are shown.}
\label{fig:ground-truth}
\end{figure*}
% \section{Rationale}
% \label{sec:rationale}
% % 
% Having the supplementary compiled together with the main paper means that:
% % 
% \begin{itemize}
% \item The supplementary can back-reference sections of the main paper, for example, we can refer to \cref{sec:intro};
% \item The main paper can forward reference sub-sections within the supplementary explicitly (e.g. referring to a particular experiment); 
% \item When submitted to arXiv, the supplementary will already included at the end of the paper.
% \end{itemize}
% 
% To split the supplementary pages from the main paper, you can use \href{https://support.apple.com/en-ca/guide/preview/prvw11793/mac#:~:text=Delete%20a%20page%20from%20a,or%20choose%20Edit%20%3E%20Delete).}{Preview (on macOS)}, \href{https://www.adobe.com/acrobat/how-to/delete-pages-from-pdf.html#:~:text=Choose%20%E2%80%9CTools%E2%80%9D%20%3E%20%E2%80%9COrganize,or%20pages%20from%20the%20file.}{Adobe Acrobat} (on all OSs), as well as \href{https://superuser.com/questions/517986/is-it-possible-to-delete-some-pages-of-a-pdf-document}{command line tools}.
